# Supplementary material for: A Local Geometric Interpretation of Feature Extraction in Deep Feedforward Neural Networks
Source: arXiv:2202.04632 source file (2022-02-10)
Supplement: Supplementary file 1 [file Appendix.tex]

%!TEX root = ./DeepNeuralNet.tex

\section{Proof of Lemma \ref{local_approximation_2}}\label{plocal_approximation_2}

Taking the first order Taylor series expansion of $\mathbf h(\mathbf d)$ at $\tilde{\mathbf d}$, we get
\begin{align}\label{e1}
\mathbf h(\mathbf d)=\mathbf h(\tilde{\mathbf d})+\tilde{\mathbf J}(\mathbf d-\tilde{\mathbf d})+o(\|\mathbf d-\tilde{\mathbf d}\|).
\end{align}
Let $\mathbf d=\mathbf W^{\operatorname{T}}\mathbf f(x)+\mathbf b$. Then, by using \eqref{constraint1}, we obtain
\begin{align}\label{e2}
\mathbf h(\mathbf W^{\operatorname{T}}\mathbf f(x)+\mathbf b)=\mathbf h(\tilde{\mathbf d})+\tilde{\mathbf J}(\mathbf W^{\operatorname{T}}\mathbf f(x)+\mathbf b-\tilde{\mathbf d})+o(\epsilon).
\end{align}
If $\mathbf d=\mathbf W^{\operatorname{T}}\bm \sigma(\tilde{\mathbf b^{(1)}})+\tilde {\mathbf d}$, we can expand $\sum_{x \in \mathcal X} P_X(x) \mathbf a_{P_{Y|X=x}}$ in \eqref{bias2} as
\begin{align}\label{e3}
&\sum_{x \in \mathcal X} P_X(x) \mathbf a_{P_{Y|X=x}}\nonumber\\
=&\mathbf h(\mathbf W^{\operatorname{T}}\bm \sigma(\tilde{\mathbf b^{(1)}})+\tilde {\mathbf d})\nonumber\\
\!\!\!=&\mathbf h(\tilde{\mathbf d})+\tilde{\mathbf J}\mathbf W^{\operatorname{T}}\bm \sigma(\tilde{\mathbf b}^{(1)})+o(\|\mathbf W^{\operatorname{T}}\bm \sigma(\tilde{\mathbf b}^{(1)})\|_2),
\end{align}
where we can design $\tilde{\mathbf d}$ and $\tilde{\mathbf b}^{(1)}$ such that $o(\|\mathbf W^{\operatorname{T}}\bm \sigma(\tilde{\mathbf b}^{(1)})\|_2)$ becomes $o(\epsilon)$.

By similar Taylor series expansion, using \eqref{constraint2}, we can get
\begin{align}\label{e4}
&\bm \sigma(\mathbf W^{(1)} \mathbf f^{(1)}(x)+\mathbf b^{(1)})\nonumber\\
=&\bm \sigma(\tilde{\mathbf b}^{(1)})+\mathbf J_1({\mathbf W^{(1)}}^{\operatorname{T}}\mathbf f^{(1)}(x)+\mathbf b^{(1)}-\tilde{\mathbf b}^{(1)})+o(\epsilon).
\end{align}

Substituting \eqref{e4} and \eqref{e3} into \eqref{e2}, we obtain
\begin{align}\label{e5}
\mathbf h(\mathbf W^{\operatorname{T}}\mathbf f(x)+\mathbf b)=&\sum_{x \in \mathcal X} P_X(x) \mathbf a_{P_{Y|X=x}}\nonumber\\
&+\tilde{\mathbf J}(\mathbf W^{\operatorname{T}}\mathbf J_1({\mathbf W^{(1)}}^{\operatorname{T}}\mathbf f^{(1)}(x)+\mathbf b^{(1)}-\tilde{\mathbf b}^{(1)}))\nonumber\\
&+\tilde{\mathbf J}(\mathbf b-\tilde{\mathbf d})+o(\epsilon).
\end{align}

By substituting \eqref{e5} into \eqref{Lemma1proofeq5} and performing similar computations  of Appendix \ref{plemma2}, we obtain \eqref{approximation1}. This concludes the proof. \textcolor{red}{Add more details}
